# Supplementary material for: Emergence of Kinship Structures and Descent Systems: Multi-level Evolutionary Simulation and Empirical Data Analysis
Source: arXiv:2105.08014 source file (2021-12-06)
Supplement: Supplementary file 1 [file clan_stat_si.pdf]

# Supplementary Information for Emergence of Kinship Structures and Descent Systems: Multi-level Evolutionary Simulation and Empirical Data Analysis

KENJI ITAO<sup>1</sup> AND KUNIHICO KANEKO<sup>\*</sup>

<sup>\*</sup>kaneko@complex.c.u-tokyo.ac.jp

## SUPPLEMENTARY TEXT

### Analytical Estimation of the Phase Diagrams of Structures

To estimate the environmental dependence of the evolved structures in Figs. 3 and 5, we calculated the fitness of each structure. We assumed that the traits and preferences in the clans would follow a multivariate normal distribution. We also assumed that the variables  $t_1, t_2, p_1$ , and  $p_2$  are independent and have the same variance  $\sigma^2$ . Thus, the probability function of the traits and preferences of the families in a certain clan (cluster), with its cluster centre at  $(t, p) = ((t_1^*, t_2^*), (p_1^*, p_2^*))$ , is given by

$$f(t_1, t_2, p_1, p_2) = \left( \frac{1}{\sqrt{2\pi\sigma^2}} \right)^4 \exp \left( -\frac{(t_1 - t_1^*)^2 + (t_2 - t_2^*)^2 + (p_1 - p_1^*)^2 + (p_2 - p_2^*)^2}{2\sigma^2} \right). \quad (S1)$$

The average values of *friend* in the same clan (kin) and, similarly, those of *rival* would be

$$\langle \text{friend}(\text{kin})^* \rangle = \int \left( \frac{1}{\sqrt{2\pi\sigma^2}} \right)^4 \exp(-|t^a - t^b|^2 / \tau^2) \quad (S2)$$

$$\exp \left( -\frac{(t_1^a - t_1^*)^2 + (t_2^a - t_2^*)^2 + (t_1^b - t_1^*)^2 + (t_2^b - t_2^*)^2}{2\sigma^2} \right) dt_1^a dt_2^a dt_1^b dt_2^b \quad (S3)$$

$$= \frac{1}{4\sigma^2/\tau^2 + 1} = \langle \text{rival}^* \rangle. \quad (S4)$$

Next, we recall that clusters emerge and are sustained depending on the fluctuation of traits and preferences. The centres of the groom and bride clans deviate with the order of the mutation rate  $\mu$ . Thus, for example, the centres of clans in dual organisations would be  $(t, p) = ((a, b), (c, d))$  and  $((b + \delta\mu, a + \delta\mu), (d + \delta\mu, c + \delta\mu))$ , (where  $\delta \sim O(1)$ ). The average values of *friend* in the mate's clan would be

$$\langle \text{friend}(\text{mate})^* \rangle = \int \left( \frac{1}{\sqrt{2\pi\sigma^2}} \right)^4 \exp(-|t^a - p^b|^2 / \tau^2) \quad (S5)$$

$$\exp \left( -\frac{(t_1^a - t_1^*)^2 + (t_2^a - t_2^*)^2 + (p_1^b - t_1^* - \delta\mu)^2 + (p_2^b - t_2^* - \delta\mu)^2}{2\sigma^2} \right) dt_1^a dt_2^a dp_1^b dp_2^b \quad (S6)$$

$$= \frac{1}{4\sigma^2/\tau^2 + 1} \exp \left( -\frac{\delta^2 \mu^2}{4\sigma^2 + \tau^2} \right). \quad (S7)$$

Then, we can estimate the value of  $\langle \text{friend} \rangle$  and  $\langle \text{rival} \rangle$ . For example, let us consider the case of dual organisation. There are two clans in the society. For each family, one clan is simultaneously kin and a rival, and the other is the mate's clan. Hence, for dual organisation,

$$\langle \text{friend} \rangle = \frac{1}{2} \langle \text{friend}(\text{kin})^* \rangle + \frac{1}{2} \langle \text{friend}(\text{mate})^* \rangle \quad (S8)$$

$$= \frac{1}{2(4\sigma^2/\tau^2 + 1)} \left( 1 + \exp \left( -\frac{\delta^2 \mu^2}{4\sigma^2 + \tau^2} \right) \right) \quad (S9)$$

$$= \frac{1}{2\beta} (1 + \exp(-\alpha\mu^2)), \quad (S10)$$

$$\langle \text{rival} \rangle = \frac{1}{2} \langle \text{rival}^* \rangle = \frac{1}{2} \frac{1}{4\sigma^2/\tau^2 + 1} = \frac{1}{2\beta}, \quad (S11)$$

where,  $\alpha = \frac{\delta^2}{4\sigma^2 + \tau^2}$ ,  $\beta = 4\sigma^2/\tau^2 + 1$ . With similar calculation, we obtained the value of  $\langle \text{friend} \rangle$  and  $\langle \text{rival} \rangle$  for each structure, as shown in Table S1.

Then, we estimated the probability of sustaining each structure. In each simulation step, the population of each clan fluctuates owing to the number of births, which follows a Poisson distribution. In addition, there is a random walk in the  $(t, \mathbf{p})$  space. Hence, if all families in the clan have no children, or all their children leave the cluster, the clan will eventually disappear. This can occur if the population is finite. We set the probability of a family not having children in their cluster to  $q$ . When there are  $N$  ( $\approx N_f$ ) families, comprising  $n$  clans in the society, the probability of sustaining the structure is  $p = 1 - nq^{N/n}$ . This increases as the number of clans  $n$  increases. As  $n$  is 1, 2, 3, and 4 for the incest structure, dual organisation, generalised exchange, and restricted exchange, respectively, the sustenance probabilities  $p_I, p_D, p_G$ , and  $p_R$  decline in this order. Additionally, as  $\mu$  decreases or  $N_f$  increases,  $p$  decreases; and as  $N_s$  increases, the probability of sampling corrupted society decreases. Hence, sustenance probability increases to 1 when  $N_f$  or  $N_s$  is large or  $\mu$  is small.

The conditions in which dual organisation is more adaptive than the incest structure are, thus, given by

$$p_I \exp\left(-d_c \cdot \left(1 - \frac{1}{\beta}\right) - d_m \cdot \frac{1}{\beta}\right) < p_D \exp\left(-d_c \left(1 - \frac{1}{2\beta} - \frac{1}{2\beta} \exp(-\alpha\mu^2)\right) - d_m \cdot \frac{1}{2\beta}\right), \quad (\text{S12})$$

$$\Leftrightarrow d_m/d_c > 1 - \exp(-\alpha\mu^2) + \frac{2}{d_c} \log p_I/p_D. \quad (\text{S13})$$

Similarly, generalised exchange is more adaptive than dual organisation if

$$d_m/d_c > 1 - \exp(-\alpha\mu^2) + \frac{6}{d_c} \log p_D/p_G. \quad (\text{S14})$$

Restricted exchange is more adaptive than generalised exchange if

$$d_m/d_c > 1 + 5 \exp(-\alpha\mu^2) + \frac{12}{d_c} \log p_G/p_R. \quad (\text{S15})$$

To be precise, we would need to calculate the average fitness of the families, rather than the average *friend* and *rival*. However, the results can be regarded as approximately equal for the rough estimations used in the current parameter regions. The boundaries between incest structure and dual organisation, dual organisation and generalised exchange, and generalised and restricted exchange asymptotically reach 0.2, 1.0, and 2.0 as  $d_c$  is small, respectively. These suggests that  $\log p_I/p_D$ ,  $\log p_D/p_G$ , and  $\log p_R/p_G$  are almost 0.1, i.e.,  $p_I/p_D \approx p_D/p_G \approx p_R/p_G \approx 1.1$ .

Thus, the above simple calculation explains the transition of emergent structures in response to the increase in  $d_m/d_c$ . In particular, if  $d_c$ ,  $N_f$ , and  $N_s$  are large, the last terms in Eq. (S13)–Eq. (S15) are negligible and the boundaries are determined by  $d_m/d_c$  (Fig. 3(A, B)). For smaller  $d_c$ , the last terms are significant, and the boundaries depend directly on  $d_m$ . As  $\mu$  increases, the factor  $\exp(-\alpha\mu^2)$  decreases, and  $p_I/p_D$ ,  $p_D/p_G$ , and  $p_G/p_R$  increase, leading to the evolution of the incest structure and dual organisation across broader parameter regions (Fig. 5(C)).

**Table S1.** The density of cooperators (*friend*), competitors (*rival*), and the probability of sustenance for each structure. Here,  $\alpha = \delta^2/(4\sigma^2 + \tau^2)$ ,  $\beta = 4\sigma^2/\tau^2 + 1$ . Distribution of  $t$  and  $\mathbf{p}$  in the clan is assumed to follow the multivariate normal distribution. Preference of brides' clan and traits of grooms' clan deviate in the order of the mutation rate  $\mu$ . For generalised and restricted exchanges, we focused on the simplest forms, that is, the number of clans were 3 and 4, respectively.

| Structure   | <i>friend</i>                                                     | <i>rival</i> | prob. |
|-------------|-------------------------------------------------------------------|--------------|-------|
| Incest      | $1/\beta$                                                         | $1/\beta$    | $p_I$ |
| Dual        | $\left(\frac{1}{2} + \frac{1}{2} \exp(-\alpha\mu^2)\right)/\beta$ | $1/2\beta$   | $p_D$ |
| Generalised | $\left(\frac{1}{3} + \frac{2}{3} \exp(-\alpha\mu^2)\right)/\beta$ | $1/3\beta$   | $p_G$ |
| Restricted  | $\left(\frac{1}{4} + \frac{1}{4} \exp(-\alpha\mu^2)\right)/\beta$ | $1/4\beta$   | $p_R$ |

## SUPPLEMENTARY FIGURES

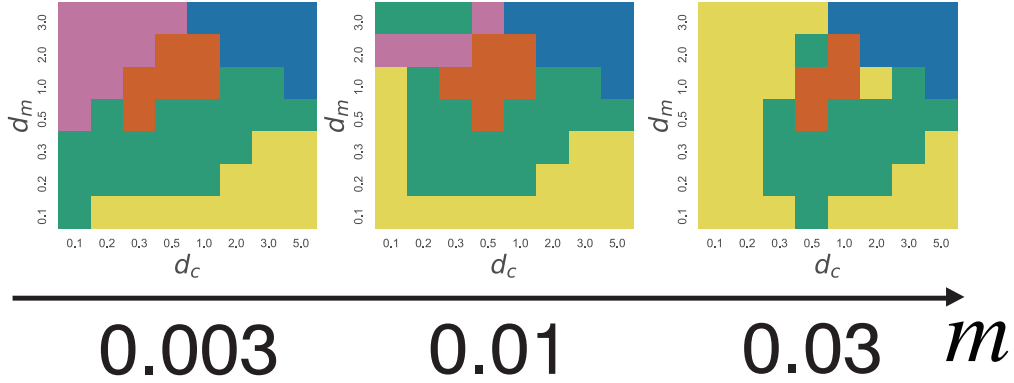

**Figure S1.** Dependence of phase diagrams of kinship structures on migration rate  $m$ . The incest structure is plotted in yellow, dual organisation in green, generalised exchange in orange, and restricted exchange in pink. Conditions leading to extinction are plotted in blue. Each family migrates to other societies with the probability of  $m$ . Phase diagram is robust against the slight migration. However, if  $m$  is large, kinship structures will become fragile, and thus sophisticated structures such as restricted or generalised exchange, will disappear. In reality, immigrants may not hold their traits and preferences, but adopt other clans' traits by belonging to some in the host society. Hence, kinship structures may be sustained for a larger migration rate.

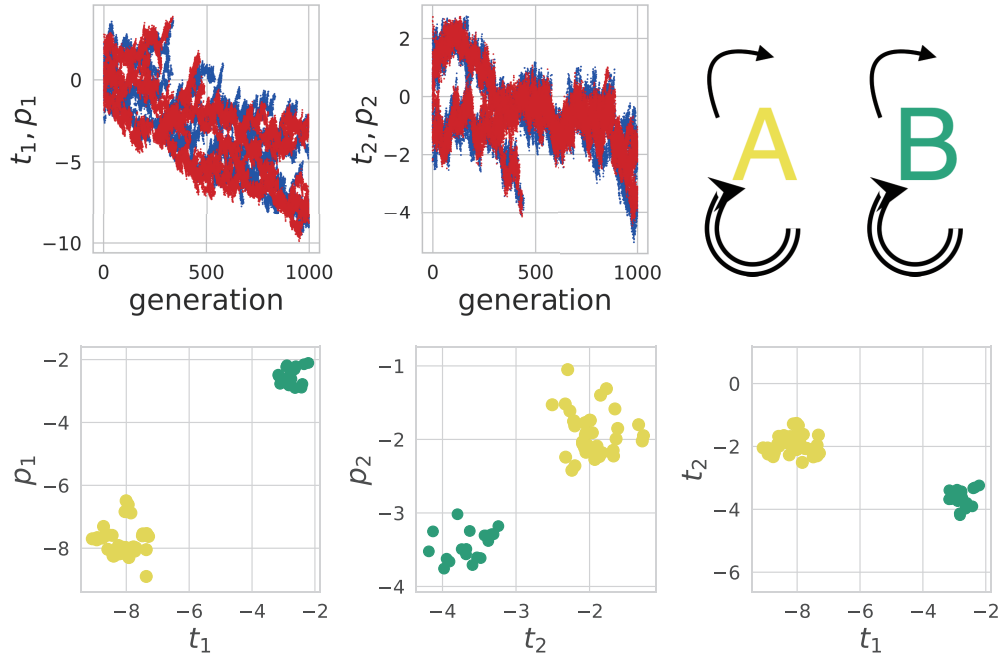

**Figure S2.** Examples of the evolution of several endogamous clans.  $(t, p)$  values of families in society after 500 simulation steps. The figures show the temporal evolution of  $(t, p)$  values (upper-left), a schematic representation of the emergent structure (upper-right), and the final state (bottom). The temporal evolution of the trait and preference values of families in society are represented in blue and red, respectively. The final states are shown as a  $t_1 - p_1$  map, a  $t_2 - p_2$  map, and a  $t_1 - t_2$  map from left to right. Here, an incest structure with two endogamous clans evolved. Marriage occurred within clan A (yellow) and B (green).  $d_c = 0.1, d_m = 0.5$ .

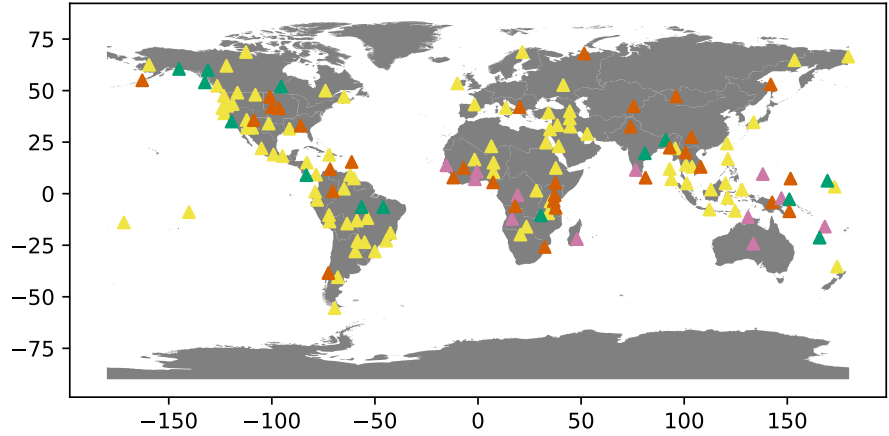

**Figure S3.** Geographic distribution of kinship structures. Incest structure, dual organisation, generalised exchange, and restricted exchange are plotted in yellow, green, orange, and pink, respectively. The information is based on [1, 2]. Kinship structures were identified in 146 of the 186 societies in the Standard Cross-Cultural Sample (SCCS). There were 87 societies identified as incest structures, 14 as dual organisation structures, 33 as generalised exchange structures, and 12 as restricted exchange structures. Each structure is globally distributed, without a clear spatial pattern. This suggests that the kinship structures in each region are achieved by cultural adaptation, rather than cultural transmission. Even though we did not analyse phylogenetic and spatial autocorrelation systematically, the large variation of kinship structures in South Asia or Oceania, for example, suggests small autocorrelation.

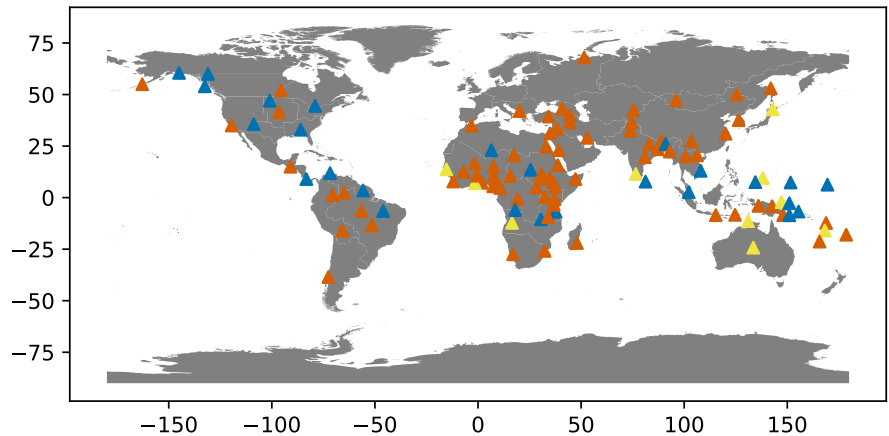

**Figure S4.** Geographic distribution of descent systems. Patrilineal, matrilineal, and double descent systems are plotted in orange, blue, and yellow, respectively. Information is based on [1, 2]. Descent systems were identified in all 186 societies in the SCCS. There were 75 societies identified as patrilineal, 26 as matrilineal, and 10 as double descent systems. Among the others, 6 were identified as ambilineal descent (i.e., descent lines were traced either paternally or maternally in each generation) and 69 as bilateral descent (i.e., relatives are recognised, but kin groups are not organised), which are omitted from the figure. Here, each descent system is globally distributed.

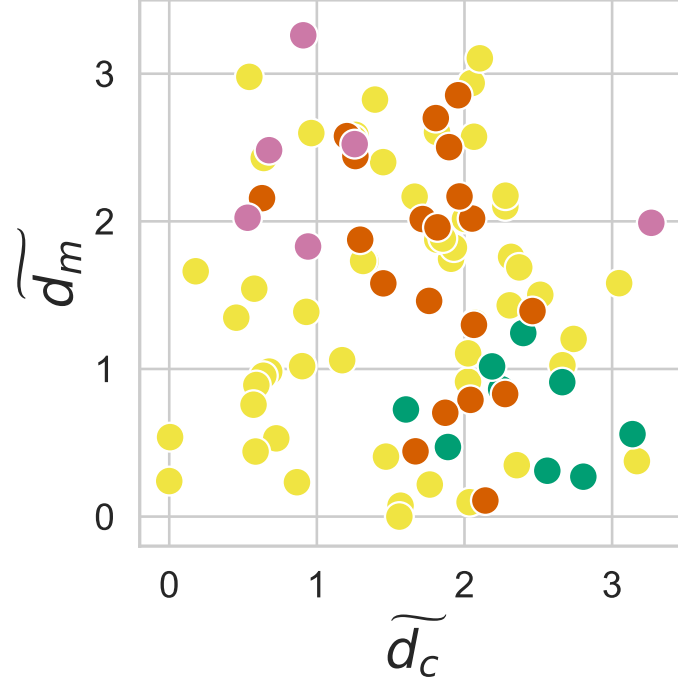

**Figure S5.** Phase diagram of the kinship structures against the parameters  $d_c$  and  $d_m$ . By analysing the SCCS, we estimated  $d_c$  and  $d_m$  for each society and plotted the dependencies of their kinship structures. The incest structure is plotted in yellow, dual organisation in green, generalised exchange in orange, and restricted exchange in pink. Incest structures are spread widely in the diagram, possibly because societies with incest structures (i.e. societies without kinship organisations) can have social organisations other than kinship influencing their adoption of these conditions.

## SUPPLEMENTARY TABLES

**Table S2.** Identification of kinship structures. We determined kinship structures by identifying the composition of clans and the descent and marriage rules between them. Here, we used the variables for exogamous units (SCCS222 and SCCS224), descent systems (SCCS70), cousin preferences for mates (SCCS230), and kinship terminologies (SCCS231). Exclusive conditions for identifying the same class are described in different rows. Exogamous units refer to the groups in which marriage is prohibited by the symbolic incest taboo, that is clans. SCCS222 (or SCCS224) = 1 indicates patrilineal (or matrilineal) endogamy and SCCS222 (or SCCS224) > 1 indicates patrilineal (or matrilineal) exogamy. The descent system refers to trait inheritance, either patrilineal, matrilineal, or double descent. SCCS70 = 1 indicates matrilineal, 2 indicates double, and 3 indicates patrilineal descent system. Marriage rules between clans can be provided by cousin preferences for mates and kinship terminology. Let us consider the woman with the largest genetic relatedness in the preferred clan: in patrilineal dual organisation, for example, a man in clan A is married to a woman in clan B. His father from A and his mother from B form a couple in A. Simultaneously, his mother's brother from B and his father's sister from A give birth to children in B. Hence, the woman with the largest genetic relatedness in clan B would be the daughter of the father's sister and mother's brother, which is a symmetrical cross-cousin. In this case, cross-cousins are differentiated from both siblings and parallel cousins, as in Iroquois terminology. If this was patrilineal generalised exchange, his father's sister would marry a man in clan C, rather than A and B. Thus, the woman with the largest genetic relatedness in clan B would be the daughter of the mother's brother, which is a matrilineal cross-cousin. In this case, mother's brother's children are equated as mother's brother or mother and father's sister's children, and are equated as sister's or own children as in Omaha terminology. SCCS230 = 1 indicates marriage preference for symmetrical cross-cousin, 2 indicates mother's brother's daughter, and 3 indicates father's sister's daughter. SCCS231 = 1 indicates Crow, 5 indicates Iroquois, and 6 indicates Omaha kinship terminology. Then, the incest structure has no exogamous units (specifically, none larger than cohabitant groups). Dual organisation is characterised by marriage prohibition within patrilineal (or matrilineal) moieties, patrilineal (or matrilineal) descent system, and mating preference for symmetrical cross-cousins. Generalised exchange is characterised by marriage prohibition within patrilineal (or matrilineal) clans, patrilineal (or matrilineal) descent system, and mating preference for the mother's brother's daughter (or father's sister's daughter), as well as Omaha (or Crow) terminology. Restricted exchange is characterised by marriage prohibition within both patrilineal and matrilineal kin, double descent system, and mating preference for symmetrical cross-cousins, as well as Iroquois terminology. Indeed, in the structure shown in Fig. 2(D), the patrilineal kin of clan  $A_1$  belong to  $A_1$  or  $A_2$ , whereas the matrilineal kin belong to  $A_1$  or  $B_1$ . This is because the character  $A$  is inherited paternally, and the number 1 is inherited maternally. Furthermore, a man in clan  $A_1$  would prefer a woman in clan  $B_2$ , who is a symmetrical cross-cousin.

| Structure            | Explanation                                                  | Criterion                         |
|----------------------|--------------------------------------------------------------|-----------------------------------|
| Incest structure     | No exogamy                                                   | "222" = "224" = 1                 |
| Dual organisation    | Patrilineal moiety exogamy                                   | "222" = 6 and "224" = 1           |
|                      | Matrilineal moiety exogamy                                   | "222" = 1 and "224" = 6           |
|                      | Patrilineal descent with symmetrical cross-cousin preference | "70" = 3, "222" > 1 and "230" = 1 |
|                      | Matrilineal descent with symmetrical cross-cousin preference | "70" = 1, "224" > 1 and "230" = 1 |
| Generalised exchange | Patrilineal descent with MoBrDa preference                   | "70" = 3 and "230" = 2            |
|                      | Patrilineal exogamy with MoBrDa preference                   | "222" > 1 and "230" = 2           |
|                      | Matrilineal descent with FaSiDa preference                   | "70" = 3 and "230" = 3            |
|                      | Matrilineal exogamy with FaSiDa preference                   | "224" > 1 and "230" = 3           |
|                      | Patrilineal exogamy with Omaha terminology                   | "222" > 1 and "231" = 6           |
| Restricted exchange  | Matrilineal exogamy with Crow terminology                    | "224" > 1 and "231" = 1           |
|                      | Exogamy concerning both patrilineal and matrilineal kins     | "222" > 1 and "224" > 1           |
|                      | Double descent with symmetrical cross-cousin preference      | "70" = 2 and "230" = 1            |
|                      | Double descent with Iroquois terminology                     | "70" = 2 and "231" = 5            |

**Table S3.** Correlation between variables in the SCCS and kinship structures. For pairs of kinship structures (dual organisation, generalised exchange, and restricted exchange), Spearman’s rank correlations between the SCCS variables and the structures were calculated. Then, the absolute values of the correlations were averaged for each pair. This table shows the variables that exhibited high correlation, together with the average of the absolute values of its correlation and the average value of the variables for each structure. The last columns show the corresponding parameters in the model. The top 10 variables in the correlation are shown above the dashed line; the five variables under the dashed line are included because they could also be relevant to the model parameters. Generally, a larger value for each item shows that the item is observed to a greater degree in societies (e.g. a large value for SCCS1737 shows that the extent of tribute payments or taxation is large). Most variables with high correlation are related to  $d_c$ ,  $d_m$ , the status of females (especially wives), or the other parameters of our model. SCCS939, SCCS983, and SCCS621 suggest that gender inequality, especially concerning wives’ status, is most frequently observed in generalised exchange compared to dual organisation or restricted exchange. As discussed in the main text, the descent system is more biased towards patrilineal descent in generalised exchange and less so in dual organisation, whereas double descent is adopted in restricted exchange. In societies with patrilineal descent systems, wives basically join husbands’ groups after marriage [3]. If male dominance is more frequently observed therein, we can explain the similarity of dual organisation to restricted exchange concerning the status of wives. However, SCCS795 suggests that the exclusion of women from the political position is most frequently observed in restricted exchange. Hence, the difference in kinship structures cannot be directly related to the gender balance in general. Regarding the other parameters, SCCS1756 is related to  $N_f$ , and SCCS1864 to  $N_s$ . The trend of SCCS1864 shows that a large (or small)  $N_s$  leads to the evolution of restricted (or generalised) exchange across larger parameter regions, which is consistent with Fig. 7. Furthermore, SCCS237 and SCCS1744 suggest that social hierarchies develop in the societies with incest structures. (Note that correlation coefficients are small because of the small variations depending on the type of kinship structures other than the incest structure.) Such social organisations can regulate social behaviours other way than kinship structures do. Hence, the trend can be related to the inconsistency of environmental dependency of the incest structures in Fig. 3. SCCS785 suggests that the migration rate  $m$  is large for the incest structure, as is consistent with the trend in Fig. S1.

| Name     | Explanation                                                         | Corr. | Incest  | Dual   | Generalized | Restricted | Model   |
|----------|---------------------------------------------------------------------|-------|---------|--------|-------------|------------|---------|
| SCCS939  | Personal Restrictions for Regular Menstruation                      | 0.65  | 4.11    | 4.75   | 5           | 2.33       |         |
| SCCS944  | Residence of the New Parents at the Birth of Their First Child      | 0.61  | 2.89    | 2.75   | 4.57        | 2          |         |
| SCCS782  | (Un) Acceptability of Violence within Society                       | 0.58  | 2.66    | 4      | 2.42        | 2.25       | $d_m$   |
| SCCS1737 | Extent of Burden Caused by Tribute Payments or Taxation             | 0.58  | 27.85   | 32     | 27          | 25.25      | $d_c$   |
| SCCS1770 | Attitude towards Violence against Other Ethnic Groups               | 0.57  | 21.53   | 30.75  | 26.25       | 20         | $d_c$   |
| SCCS768  | (No) Conflict between Communities of the Same Society               | 0.55  | 2.55    | 3.29   | 2           | 1.5        | $d_m$   |
| SCCS1120 | Some External War                                                   | 0.54  | 0.84    | 1      | 0.89        | 0.25       | $d_c$   |
| SCCS173  | Rape                                                                | 0.53  | 2.7     | 1      | 3.25        | 3.5        | $d_m$   |
| SCCS773  | (No) Internal Warfare                                               | 0.52  | 2.68    | 3.57   | 1.92        | 1.5        | $(d_c)$ |
| SCCS973  | Degree of Marriage Celebration                                      | 0.52  | 2.79    | 3      | 2.86        | 4          |         |
| SCCS961  | Restrictions on Premarital Sex                                      | 0.51  | 4.04    | 2      | 3.38        | 4.75       | $d_m$   |
| SCCS983  | Financial Loss by the Wife after Divorce                            | 0.48  | 2.95    | 4      | 4.4         | 3.5        |         |
| SCCS788  | Cross-cutting Ties                                                  | 0.45  | 1.65    | 2.57   | 1.93        | 1.5        | $d_c$   |
| SCCS1772 | Hostility towards Other Ethnic Groups                               | 0.45  | 31.97   | 37.4   | 29.4        | 20.4       | $d_c$   |
| SCCS1725 | Possibility for Peaceful Territorial Expansion                      | 0.43  | 15.17   | 14.2   | 18          | 21         |         |
| SCCS795  | (Low) Gender Differences in Political Positions of Authority        | 0.42  | 2.82    | 2.67   | 3.38        | 4          |         |
| SCCS960  | Violation of the Incest Taboo                                       | 0.41  | 2.68    | 2      | 2.25        | 4.25       | $d_m$   |
| SCCS1756 | Size of Local Community                                             | 0.32  | 3407.59 | 186.67 | 229.88      | 96.67      | $N_f$   |
| SCCS1864 | Number of Societies within 100 Mile Radius                          | 0.22  | 1.07    | 0.5    | 1.58        | 1.83       | $N_s$   |
| SCCS621  | (No) Explicit View That Men Dominate Their Wives                    | 0.18  | 1.46    | 1.57   | 1.2         | 1.25       |         |
| SCCS237  | Jurisdictional hierarchy beyond local community                     | 0.14  | 2.08    | 1.5    | 1.82        | 1.92       |         |
| SCCS1744 | Lower Level Participation in Decision Making of Political Authority | 0.13  | 1.9     | 2.43   | 2.39        | 2.25       |         |
| SCCS785  | (No) Local Political Fission of Dissatisfied Persons                | 0.10  | 1.46    | 2.2    | 1.92        | 2.0        | $m$     |

### **Values of SCCS Variables Used for Data Analyses**

The values of SCCS variables are explained as below, according to [1, 2, 4–15]

#### **SCCS70 Descent - Membership in Corporate Kinship Groups**

1. Matrilineal—through female line, 2. Double descent—separate groups through male and female lines, 3. Patrilineal—through male line, 4. Ambilineal—through one parent in each generation, and 5. Bilateral—not a corporate kin group.

#### **SCCS222 Largest patrilineal exogamous group [Note, identical to EA018]**

1. No exogamy, 2. Extended taboo, 3. Lineages, 4. Sibs, 5. Phratries, and 6. Moieties.

#### **SCCS224 Largest matrilineal exogamous group [Note, identical to EA020]**

1. No exogamy, 2. Extended taboo, 3. Lineages, 4. Sibs, 5. Phratries, and 6. Moieties.

#### **SCCS230 Cousin marriages preferred: subtypes [Note, identical to EA026]**

1. Symmetrical cross-cousin, 2. Mother's brother's daughter, 3. Father's sister's daughter, 4. Father's brother's daughter, 5. Second cousin, and 9 None preferred.

#### **SCCS231 Kin terms for cousins [Note, identical to EA027]**

1. Crow, 2. Descriptive, 3. Eskimo, 4. Hawaiian, 5. Iroquois, 6. Omaha, 7. Sudanese, 8. Mixed.

#### **SCCS939 Personal Restrictions or Regular Menstruation**

1. No restriction during this period, 2. Restrictions on personal activities but not social activities, 3. Restrictions on personal and social movements, 4. Few restrictions placed on personal and social activities, 5. Moderate restrictions (may not cook), and 6. Severe restrictions – secluded in a menstrual hut.

#### **SCCS944 Residence of the New Parents at the Birth of Their First Child**

1. Temporary matrilocality, 2. Permanent matrilocality, 3. Ambilocality, 4. Neolocality, and 5. Patrilocality.

#### **SCCS782 (Un) Acceptability of Violence toward Members of the Same Society, but outside the Local Community**

1. Valued, 2. Acceptable, 3. Tolerated, and 4. Disapproved.

#### **SCCS1737 Extent of Burden Caused by Tribute Payments or Taxation**

20. Sporadic taxation or request for tribute, 21. Sporadic exactions are reported not to be burdensome, 22. Sporadic exactions are reported to be burdensome, 30. Regular taxation or request for tribute, 31. Regular exactions are reported not to be burdensome, and 32. Regular exactions are reported to be burdensome.

#### **SCCS1770 Attitude towards Physical Violence against Members of Other Ethnic Groups**

10. Physical violence outside of ethnic group is rejected, 11. Physical violence outside of ethnic group is rejected because of military inferiority or cowardice, 20. Physical violence is tolerated or accepted—specification of the enemies is absent, 21. Physical violence is tolerated or accepted but not against the majority of other ethnic groups, 22. Physical violence is tolerated or accepted against the majority of other ethnic groups, 30. Physical violence is appreciated—no further specification against whom, 31. Physical violence is appreciated but not against the majority of other ethnic groups, and 32. physical violence is appreciated against the majority of other ethnic groups.

#### **SCCS768 (No) Conflict between Communities of the Same Society**

1. Endemic, 2. High, 3. Moderate, and 4. Mild or rare.

#### **SCCS1120 Some External War (Ott: 143-49 Variables 5, 6)**

0. Absent, and 1. Present.

#### **SCCS173 Rape**

1. Accepted/ignored, 2. Ridiculed, 3. Mildly disapproved, and 4. Strongly disapproved.

#### **SCCS773 (No) Internal Warfare (between Communities of Same Society)**

1. Frequent, occurring at least yearly, 2. Common, at least every five years, 3. Occasional, at least every generation, and 4. Rare or never.

**SCCS973 *Personal Restrictions or Regular Menstruation***

1. No celebration, 2. Small celebration, 3. Moderate celebration, and 4. Elaborate celebration.

**SCCS961 *Restrictions on Premarital Sex***

1. It is permitted for both sexes, 2. It is permitted for both sexes, but in limited contexts, e.g., with prostitutes or as part of a ceremony, 3. It is permitted and not punished unless pregnancy results, 4. It is permitted for males but not for females, 5. Premarital relations are disapproved but infrequent, 6. Insistence on virginity for the women. There is no information on restrictions on the male, and 7. Premarital relations are strongly disapproved and rare.

**SCCS983 *Property Exchanges after Divorce. Ranked in order of the amount of financial loss incurred by the wife when a divorce occurs***

1. There is no divorce, 2. No financial transaction occurs after a divorce (equal share), 3. The husband or his kin pay compensation, 4. The transaction that occurs depends on the circumstances, and 6. The wife and/or her kin group pay compensation.

**SCCS788 *Cross-cutting Ties: Extent to Which Individuals Living in Different Communities of the Same Society Linked Together in Politically Relevant Ways***

1. No politically relevant links, formal organizations, or strong informal obligations which extend beyond the local community, 2. Some politically relevant ties, but wider society divided into some discrete groups not linked through cross-cutting ties, 3. Cross-cutting ties link individuals throughout the society, cutting across territorial groups in one or more ways.

**SCCS1772 *Hostility towards Other Ethnic Groups***

10. No or negligible hostility, 20. Weak degree of hostility, 30. Moderate degree of hostility, 31. Moderate degree of hostility only directed against certain other ethnic groups, 32. Moderate degree of hostility directed against almost all other ethnic groups, 40. High degree of hostility, 41. High degree of hostility only directed against certain other ethnic groups, and 42. High degree of hostility directed against almost all other ethnic groups

**SCCS1725 *Possibility for Peaceful Territorial Expansion***

10. peaceful territorial expansion impossible, 20. peaceful territorial expansion possible, no information on quality of land, 21. access to land of good quality, and 22. access to land of restricted quality.

**SCCS795 *Gender Differences in Political or Quasi-political Positions of Authority***

1. Women and men eligible for some of the same positions and women commonly do so, 2. Women and men eligible for some of the same positions and women occasionally do so, 3. Women rarely, if ever, hold some of the same positions regardless of rules of eligibility, and 4. The same political positions are not open to both women and men.

**SCCS960 *Violation of the Incest Taboo***

1. None or mild punishment, 2. Moderate punishment, 3. Severe punishment, 4. Punishment to those other than the offenders, 5. Punishment to the whole social group, and 6. Punishment that affects the offenders and their social group.

**SCCS1756 *Size of Local Community***

Population of local community

**SCCS1864 *Concordance: Number of Societies within 100 Mile Radius***

The number of societies within a 100-mile radius

**SCCS621 *(No) Explicit View That Men Should and Do Dominate Their Wives***

1. Yes, 2. No, evidence of rough equality, and 3. No, evidence of wife dominance.

**SCCS237 *Jurisdictional hierarchy beyond local community [Note, identical to EA033]***

1. No political authority beyond community (e.g., autonomous bands and villages), 2. One level (e.g., petty chiefdoms), 3. Two levels (e.g., larger chiefdoms), 4. Three levels (e.g., states), and 5. Four levels (e.g., large states).

**SCCS1744 *Lower Level Participation in Decision Making of the Unit of Maximal Political Authority*** 1. decision making at the highest level of political authority independent of lower-ranking levels, groups, or individuals, 2. decisions at the highest level of political authority are made after consultation with representatives of lower-ranking levels, groups, or individuals, and 3. lower-ranking individuals or group representatives fully participate in decision making at the highest level of political authority, they are members of the decision-making body.

**SCCS785 (No) *Local Political Fission of Dissatisfied Persons*** 1. Often move to another community following disputes, 2. Sometimes move to another community following disputes, and 3. Rarely or never move to another community following disputes

## REFERENCES

1. G. P. Murdock and D. R. White, "Standard cross-cultural sample," *Ethnology* **8**, 329–369 (1969).
2. K. R. Kirby, R. D. Gray, S. J. Greenhill, F. M. Jordan, S. Gomes-Ng, H.-J. Bibiko, D. E. Blasi, C. A. Botero, C. Bowern, C. R. Ember *et al.*, "D-place: A global database of cultural, linguistic and environmental diversity," *PloS one* **11**, e0158391 (2016).
3. E. Service, *Primitive Social Organization: An Evolutionary Perspective*, Random House studies in anthropology (Random House, 1962).
4. J. P. Gray, "A corrected ethnographic atlas," *World Cult.* **10**, 24–85 (1999).
5. G. P. Murdock, "Ethnographic atlas, installments i-xxvii," *Ethnology* pp. 1–10 (1962).
6. D. R. White and M. L. Burton, "Causes of polygyny: Ecology, economy, kinship, and warfare," *Am. Anthropol.* **90**, 871–887 (1988).
7. G. J. Broude and S. J. Greene, "Cross-cultural codes on twenty sexual attitudes and practices," *Ethnology* **15**, 409–429 (1976).
8. S. G. Frayser, *Varieties of sexual experience: An anthropological perspective on human sexuality* (HRAF Press, 1985).
9. M. H. Ross, "Political decision making and conflict: Additional cross-cultural codes and scales," *Ethnology* **22**, 169–192 (1983).
10. H. Lang, "Conan: An electronic code-text data-base for cross-cultural studies," *World Cult.* **9**, 13–56 (1998).
11. V. W. Nammour, "Drums and guns: A cross-cultural study of the nature of war," Unpubl. doctoral dissertation, Univ. Or. (1974).
12. C. R. Ember and M. Ember, "Warfare, aggression, and resource problems: Cross-cultural codes," *Behav. Sci. Res.* **26**, 169–226 (1992).
13. P. C. Rosenblatt, R. P. Walsh, and D. A. Jackson, *Grief and mourning in cross-cultural perspective* (HRAF press, 1976).
14. R. P. Rohner and E. C. Rohner, "Parental acceptance-rejection and parental control: Cross-cultural codes," *Ethnology* **20**, 245–260 (1981).
15. R. P. Rohner and E. C. Rohner, "Enculturative continuity and the importance of caretakers: Cross-cultural codes," *Behav. Sci. Res.* **17**, 91–114 (1982).
